# Supplementary material for: Trading Complexity for Sparsity in Random Forest Explanations
Source: arXiv:2108.05276 source file (2021-08-11)
Supplement: Supplementary file 1 [file additional.tex]

%%%%%%%%%%%%%%%%%%%%%%%%%%%%%%%%%%%%%%%%%%%%%%%%%%%%%%%%%%%%%%%%%%%%%%%%%%%%%%%%
\section{Additional Results}\label{additional}
%%%%%%%%%%%%%%%%%%%%%%%%%%%%%%%%%%%%%%%%%%%%%%%%%%%%%%%%%%%%%%%%%%%%%%%%%%%%%%%%

%\paragraph{Minimal reasons.} Si on n'a pas la place on remet des paragraphes. Sinon les sous-section étant relativement longues, c'est plus lisible.

\subsection{Comprehensible Reasons}

%\paragraph{Comprehensible reasons.}  

Sufficient reasons are not always guaranteed to be ``intelligible''. 
Indeed, it can be the case that some features in the prime implicant 
are not understandable by the user to which the explanation is supplied. 
This calls for a notion of \emph{comprehensible reason}:

% Fred: l'exemple médical est intéressant, mais pas sûr qu'on ait la place.
% In some cases, limiting the size of an explanation to a few literals is not enough 
% to ensure that the explanation is intelligible \cite{CosteMarquis20}.
% Indeed, it can be the case that some of the features in the explanation are not understandable by the user to which the explanation
% must be reported. 
%This happens, for example, when trying to predict diseases from observed symptoms and physiological measures
%associated with patients: though the fact that the erythrocyte sedimentation rate in a blood test is over a given threshold is a
%meaningful piece of information for a physician, for many people this will be meaningless.

\begin{definition}[Comprehensible Reason] 
    Let $f \in \mathcal F_n$ and $\vec x \in \{0,1\}^n$ such that $f(\vec x) = 1$.
    In addition, let $I \subseteq X_n$ be a subset of intelligible features. 
    Then, a \emph{comprehensible reason} for $\vec x$ given $f$ and $I$ is a sufficient reason for $\vec x$ given $f$ that contains only literals built up from $I$.
\end{definition}

\begin{example} Suppose that the user does not understand what \emph{sympodial}\footnote{An orchid is sympodial when it grows sideways.} (feature $x_4$) means.
 Is it possible to find a sufficient reason for $\vec x$ given $T$ that does not include $x_4$? 
    Obviously, the answer is negative because $x_4$ is \emph{mandatory} for the {\it Cattleya} classifier $T$, that is, any sufficient reason 
    for any input instance must include a literal on $x_4$. 
\end{example}

As illustrated in the above example, a key issue for deriving ``intelligible'' reasons is to determine whether at least one comprehensible reason exists, 
depending on the choice of $I$. Interestingly, this problem is tractable for decision trees, and even for random forests: 

\begin{proposition} \label{prop:understandablereasonRF}
    Let $F \in \rf_{n, m}$ and $\vec x \in \{0,1\}^n$ such that $F(\vec x) = 1$. 
    Then, for any set $I \subseteq X_n$ of intelligible features, deciding whether a comprehensible reason for $\vec x$ given $F$ and $I$
    exists, and deriving such a reason when this is the case, can be done in $\mathcal O(n \size{F})$ time.
\end{proposition}

%\fred{Est-ce qu'on pourrait generaliser aux delta-probable comprehensible reasons? ... Cela reste poly, mais c'est une consequence de 3 \& 4.}
%\pierre{Oui, j'ai ajouté une phrase dans la partie "Probabilistic Reasons"}

%\color{blue}
%\pierre{J'ai remis la suite (partie en bleu). Merci de le mettre éventuellement en commentaires mais de ne pas l'effacer sinon cela m'oblige à retaper
%des trucs et je risque d'introduire des erreurs.}
%\fred{OK Pierre}

\subsection{Inclusion-Preferred Reasons}

%\fred{Pierre, si l'on a la place je suggere de mettre les raisons preferees au sens lexicographique (donc le modele LPM) 
%ainsi que les raisons preferees au sens lineaire additif (donc le modele APM). Sinon on se focalise sur LPM, où le resultat est poly. }

The user may also have some expectations about the features that should be present in explanations. 
For instance, she might consider that some features are more important than others for explaining decisions. 
The reason that is derived should cohere as much as possible to the user's expectations or \emph{confirmation bias}.\footnote{Confirmation bias is the tendency to search for, 
interpret, favor, and recall information in a way that confirms or supports one's prior beliefs or values. Since the 1960's, many experiments in psychology and cognitive science 
people have shown that people are biased toward confirming their existing beliefs (see e.g., \cite{Oswaldetal04}).}
However, when computing a sufficient reason, even a comprehensible one, we cannot guarantee that a ``better'' reason 
for the user would not exist. 

To make it more formal, one needs a notion of \emph{``preferred''} sufficient reason. Depending on the preference model at hand, the
computation of a single preferred reason can be intractable (as we will see soon). Fortunately, there are preference models for which
intractability can be avoided. 
 Especially, this is the case when the preference relation is ordinal and based on a total preorder $\leq$ over $X_n$,
 such that $x_i \leq x_j$ means that feature $x_i$ is considered as less important or less expected than feature $x_j$. 
 $\leq$ can be represented by a \emph{prioritization} (or stratification) of $X_n$, i.e., 
 an ordered partition $C_1, \ldots, C_p$ of the features from $X_n$ such that $x_i$ and $x_j$ belongs to the
 same set of the partition if and only if $x_i \leq x_j$ and $x_j \leq x_i$, and $C_i$ precedes $C_j$ in the partition (i.e., $i < j$) whenever
 every element of $C_i$ is before every element of $C_j$ w.r.t. $\leq$. Whatever $C$ among $C_1, \ldots, C_p$ and a term $t$ over $X_n$,
 $t[C]$ denotes the term composed of the literals of $t$ that are over variables from $C$.

 Based on the prioritization $C_1, \ldots, C_p$ of $X_n$ induced by $\leq$, one can define a preference relation $\sqsubset$ on the terms 
 over $X_n$ by stating that $t \sqsubset t'$ if and only if $\exists i \in \{1, \ldots, p\} \forall j \in \{1, \ldots, i-1\}$, $t[C_j] = t'[C_j]$ and 
 $t[C_i] \subset t'[C_i]$.\footnote{The construction is reminiscent to the one used for characterizing preferred subtheories in \cite{Brewka89}.}
 It can be checked that $\sqsubset$ is a strict, partial order (i.e., an irreflexive and transitive relation). 
 Given a set of terms, the minimal ones w.r.t. $\sqsubset$ correspond intuitively to those that contain as few unexpected literals
 as possible (where the comparison is based on set inclusion). On this ground, we are now ready to define the notion of inclusion-preferred reason:
 
\begin{definition}[Inclusion-Preferred Reason] 
    Let $f \in \mathcal F_n$, $\leq$ a total preorder over $X_n$, and $\vec x \in \{0,1\}^n$ be an instance such that $f(\vec x) = 1$.
    Then, an \emph{inclusion-preferred reason} for $\vec x$ given $f$ is a sufficient reason $t$ for $\vec x$ given $f$ 
    such that there is no sufficient reason $t'$ for $\vec x$ given $f$ satisfying $t' \sqsubset t$.
\end{definition}

\begin{example}[Example \ref{running-ex} cont'ed]
Suppose that the expectations of the explainee correspond to the prioritization $\{x_4\}, \{x_3, x_2\}, \{x_5\}, \{x_1\}$ reflecting the fact
that having fragrant flowers is, for her/him, a more salient aspect of {\it Cattleya} orchids than the other features.
% (especially than $d$ that she/he does not understand). 
Then $x_1 \wedge x_4$ is an inclusion-preferred reason for $\vec x$ given $T$, while $x_2 \wedge x_3 \wedge x_4$ is not because 
$x_1 \wedge x_4 \sqsubset x_2 \wedge x_3 \wedge x_4$ holds.
\end{example}

The greedy algorithm presented above for generating one sufficient reason can be cast in such a way that it generates
an inclusion-preferred reason for an instance given a decision tree, or more generally a random forest:

\begin{proposition} \label{prop:favoritereasonRF}
    Let $F \in \rf_{n,m}$, $\leq$ be a total preorder over $X_n$, and $\vec x \in \{0,1\}^n$. 
    Then, deriving an inclusion-preferred reason for $\vec x$ given $F$ and $\leq$ can be done in $\mathcal O(\size{G} + n \size{F})$ time
    where $G$ is the graph $(X_n, \leq)$.
\end{proposition}

\subsection{Minimal Reasons}

As conciseness is often a desirable property of explanations, a natural way for improving the clarity of 
sufficient reasons is to focus on those of minimal size:

\begin{definition}[Minimal Reason] 
    Let $f \in \mathcal F_n$ and $\vec x \in \{0,1\}^n$ such that $f(\vec x) = 1$.
    A \emph{minimal reason} for $\vec x$ given $f$ is a sufficient reason for $\vec x$ given $f$ that contains a minimal number
    of literals.
\end{definition}

\begin{example} Based on our running example, $x_1 \wedge x_4$ is a minimal reason for $\vec x$ given $T$, 
    while $x_2 \wedge x_3 \wedge x_4$ is not.
\end{example}

Importantly, \emph{minimal reasons} should not to be confused with \emph{minimum-cardinality explanations}  \cite{ShihCD18},
where the minimality condition bears on the features set to $1$ in the input instance. 
%As a direct by-product of Proposition 8 from \cite{Audemardetal20}, 
%computing a minimum-cardinality explanation for an input instance $\vec x$ given a decision tree $T$
%can be done in polynomial-time. Unfortunately, this is not the case for minimal reasons, 
%which are computationally more demanding:
The computation of a minimal reason looks more demanding than the computation of a sufficient reason, even 
for the case of decision trees:

\begin{proposition}\label{prop:minimalreasonDT}
    Let $F \in \rf_{n,m}$ and $\vec x \in \{0,1\}^n$ such that $F(\vec x) = 1$.
%    Unless {\sf P = NP}, there is no polynomial-time algorithm for computing a minimal reason for $\vec x$ given $F$,
%    even when $F = \{T\}$ reduces to a single decision tree.
    Computing a minimal reason for $\vec x$ given $F$ is {\sf NP}-hard, 
    even when $F = \{T\}$ reduces to a single decision tree.
\end{proposition}

Obviously enough, this {\sf NP}-hardness result can be extended from minimal reasons to the more general concept of a minimal-weight reason.\footnote{A minimal 
reason is a minimal-weight reason whenever $w$ is a constant mapping from $X_n$ to $\mathbb{N}^*$.} 

\begin{definition}[Minimal-Weight Reason] 
    Let $f \in \mathcal F_n$ and $\vec x \in \{0,1\}^n$ such that $f(\vec x) = 1$. Let $w: X^n \rightarrow \mathbb{N}^*$ be a weight mapping
    associating with every feature a positive integer.
    A \emph{minimal-weight reason} for $\vec x$ given $f$ and $w$ is a sufficient reason $t$ for $\vec x$ given $f$ that minimizes
    $\Sigma_{x \in \Var{t}} w(x)$.
\end{definition}

$w$ can be interpreted as a cardinal preference over the features. When the explainee has such a preference in mind, it makes sense to lift it 
to terms (and reasons) by summing the weight (disutility) of the features occurring in the terms (and reasons).

Interestingly, computing a minimal-weight reason given a random forest and a weight mapping can be achieved by solving an instance of the
\textsc{Weighted Partial MaxSAT} problem:
%{\sf NP}-optimization problem:

\begin{proposition}\label{prop:minimaloptim}
    Let $F \in \rf_{n,m}$ and $\vec x \in \{0,1\}^n$ such that $F(\vec x) = 1$. Let $w: X^n \rightarrow \mathbb{N}^*$ be a weight mapping.
    A minimal-weight reason for $\vec x$ given $F = \{T_1, \ldots, T_m\}$ and $w$ consists of the literals shared by 
   $t_{\vec x} = \bigwedge_{i=1}^n \ell_i$ and  $t_{\vec v^*}$ where $\vec v^*$ is a solution of the instance of the 
   \textsc{Weighted Partial MaxSAT} problem given by the following multiset of weighted clauses:
   $$\{(\overline{x_i}, w(x_i)) \mid x_i(\vec x) = 1\} \cup \{(x_i, w(x_i)) \mid x_i(\vec x) = 0\}$$ 
   $$\cup \{(c, \infty) \mid c \in \cnf(\Sigma_{j=1}^m s_j > \frac{m}{2})\} \cup$$ 
   $$ \{(\overline{s_j} \vee c[\vec x], \infty) \mid  j \in [m] \mbox{ and } c \in \cnf(T_j)\}.$$
%    
%\noindent $\mathtt{Determine \: } \vec x^* \in \{0,1\}^n$\\
%\noindent $\mathtt{minimizing \: } \Sigma_{i=1}^n \mathit{sign}(\ell_i) \cdot w(x_i) \cdot x_i$\\
%\noindent $\mathtt{provided \: that}$\\
%\noindent $\Sigma_{j=1}^m s_j > \frac{m}{2}$\\
%\noindent $\overline{s_j} \vee c[\vec x] \mathtt{\: for \: every \: } j \in [m] \mathtt{\: and \: every \: } c \in \cnf(T_j)$
\end{proposition}

Let us recall that a \textsc{Weighted Partial MaxSAT} instance consists of a set of weighted clauses, where weights are
integers (the corresponding clauses are called soft clauses) or $\infty$ (the corresponding clauses are called hard clauses).
In the \textsc{Weighted Partial MaxSAT} instance presented in Proposition \ref{prop:minimaloptim}, $\cnf(\Sigma_{j=1}^m s_j > \frac{m}{2})$
denotes any \cnf\ encoding\footnote{Many such encodings exist, see \cite{DBLP:conf/cp/Sinz05,DBLP:journals/constraints/AsinNOR11}} of the cardinality constraint 
$\Sigma_{j=1}^m s_j > \frac{m}{2}$, where each $s_j$ ($j \in [m]$) is a selector variable associated with the decision tree $T_j$ of $F$. 
A solution of this instance is an assignment $\vec v^*$ of the variables occurring
in the clauses (here, variables from $X_n \cup \{s_j \mid j \in [m]\}$ plus the auxiliary variables used in the encoding of the cardinality constraint, if any)
that minimizes the sum of the weights of the clauses that are violated.

Interestingly, many algorithms for \textsc{Weighted Partial MaxSAT} have been designed during the past decade (see \cite{DBLP:journals/ai/AnsoteguiG17} 
for a presentation of the main ones). Thanks to Proposition \ref{prop:minimaloptim}, we can take advantage of them for computing minimal reasons and 
minimal-weight reasons.

As an alternative to \textsc{Weighted Partial MaxSAT} solving, we can find good approximations of minimal reasons using the following greedy covering algorithm:
starting from $t = \emptyset$, iteratively add to $t$ a vertex $l_i \in t_{\vec x}$ of maximal degree $\mathrm{deg}(l_i)$, and removes it together with all 
adjacent hyperedges in $H_{\vec x}(T)$. Let $\mathrm{adj}(l_i)$ be the set of vertices in $H_{\vec x}(T)$ which are adjacent to $l_i$, 
and let $A = \max_{i=1}^n \size{\mathrm{adj}(l_i)}$. Note that for the \cnf\ encoding of decision trees, 
$A$ often coincides with the depth of the tree. Based on the analysis of greedy covering algorithm \cite{SLAVIK1997,OKUN2005}, we get the following result. 

\begin{proposition}\label{prop:approximable}
    Given $T \in \dt_{n}$ and $\vec x \in \{0,1\}^n$ such that $T(\vec x) = 1$, the problem of finding 
    a minimal reason for $\vec x$ with respect to $T$ is approximable to within a ratio of $\min(A/2 + 1, \ln n - \ln\ln n + \Theta(1))$. 
\end{proposition}

Unfortunately, this result does not extend to the case of random forests. \pierre{Write a proposition that states it formally}

Finally, a direct consequence of Proposition \ref{prop:minimalreasonDT} is that the greedy algorithm used for pointing out in polynomial time a sufficient reason 
cannot be extended to the issue of selecting a ``preferred'' reason from the sufficient ones when any preference relation is considered. 
%Especially, as we will see next, computing a reason that contains as few features
%as possible cannot be achieved in polynomial time unless {\sf P = NP}. The search for a ``preferred reason''
%among the sufficient reasons cannot always be done efficiently. 
Note that a straightforward generate-and-test algorithm would not be not
convenient to reach the goal because the search space (i.e., the set of all sufficient reasons) is of exponential size
in the worst case.
%For the classes of \cnf\ and \dnf\ formulas, it is well-known that an input instance can have exponentially many sufficient reasons.
%For example, the monotone \cnf\ formula $F = \bigwedge_{i=1}^{\lfloor\frac{n}{2}\rfloor} (x_{2i-1} \vee x_{2i})$ has $2^{\lfloor\frac{n}{2}\rfloor}$.
%prime implicants, each of them being implied by $\vec x = (1,1,\cdots,1)$. Surprisingly, 
Indeed, even for the restricted class of decision trees of 
logarithmic depth, an input instance can have exponentially many sufficient reasons:

\begin{proposition}\label{prop:nbDT}
    Let $\dt^k_{n}$ be the class of decision trees of depth $k \geq 1$ over $n = 2^k - 1$ variables. Then, there is a decision tree $T \in \dt^k_{n}$ 
    such that for any $\vec x \in \{0,1\}^n$, the number of sufficient reasons for $\vec x$ given $T$ is at least $\lfloor \frac{3}{2}^{\frac{n + 1}{2}} \rfloor$. 
\end{proposition}

%\paragraph{Probabilistic Reasons.} 

\subsection{Probabilistic Reasons}

A natural way to circumvent the computational barrier of finding minimal reasons is to rely on a probabilistic notion of prime implicant explanations,
as suggested in \cite{WALDCHEN2020}. This leads to generalize the notion of sufficient reasons, instead of refining it.
Basically, the idea of ``probabilistic`'' prime implicants stems from the fact that standard, ``logical'' prime implicants 
are often too rigid for high dimensional, and possibly noisy, classification tasks. Thus, by forgetting few models of the classifier $f$, 
probabilistic prime implicants may provide much shorter explanations. Formally, let $\PP_{\vec z}[f(\vec z)]$ be the probability 
that an assignment $\vec z$, drawn at random according to the uniform distribution over $\{0,1\}^n$, is a model of $f$, i.e.
\begin{align*}
\PP_{\vec z}[f(\vec z)] = \frac{\size{\vec z \in \{0,1\}^n: f(\vec z) = 1}}{\size{\vec z \in \{0,1\}^n}}
\end{align*}
Now, let $\PP_{\vec z}[f(\vec z) \mid t \subseteq t_{\vec z}]$ be the conditional probability that a random assignment $\vec z$ is a model of $f$, 
given that $\vec z$ is an extension of $t$:
\begin{align*}
   \PP_{\vec z}[f(\vec z) \mid t \subseteq t_{\vec z}] = \frac{\size{\vec z \in \{0,1\}^n: f(\vec z) = 1 \mbox{ and } t \subseteq t_{\vec z}}}{\size{\vec z \in \{0,1\}^n: t \subseteq t_{\vec z}}}
\end{align*}
For a confidence parameter $\delta \in [0, 1]$, a term $t$ is called a $\delta$-\emph{probable implicant} of $f$ if $\PP_{\vec z}[f(\vec z) \mid t \subseteq t_{\vec z}] \geq \delta$, 
that is, the proportion of extensions of $t$ that are models of $f$ is at least $\delta$. If $t$ is a $\delta$-probable implicant of $f$ and no proper subset of $t$ 
is a $\delta$-probable implicant of $f$, then $t$ is called a $\delta$-\emph{probable prime implicant} of $f$.

\begin{definition}[$\delta$-Probable Reason] 
    Let $f \in \mathcal F_n$ and $\vec x \in \{0,1\}^n$ such that $f(\vec x) = 1$.
    A \emph{$\delta$-probable reason} for $\vec x$ given $f$ is a $\delta$-probable prime implicant $t$ of $f$ such that $t \subseteq t_{\vec x}$.
\end{definition}

\begin{example}
    Based on our running example, we can observe that $x_2 \land x_4$ is not a sufficient reason for $\vec x$ given $T$, but it is
    still a $75\%$-probable reason for $\vec x$ (given $T$).
\end{example}
    
Clearly enough, considering $\delta$-probable reasons can also be a way to get rid of incomprehensible characteristics in sufficient reasons
(even if there is no guarantee that incomprehensible characteristics are systematically removed).

Finding $\delta$-probable reasons is an ${\sf NP^{PP}}$-\pierre{hard} problem (see Theorem 2.4 in \cite{WALDCHEN2020}). 
However, this problem can be shown as tractable for decision trees via slightly modifying the greedy algorithm for sufficient reasons. Namely, at each iteration $i \in [n]$, 
instead of testing whether the current term $t$, deprived from the literal $l_i$, is an implicant of $T$, we check whether $t \setminus \{l_i\}$ is a $\delta$-probable implicant 
of $T$. Using the fact that conditioning and model counting operations can be done in linear time for decision trees \cite{Koricheetal13}, the inequality 
$\PP_{\vec z}[f(\vec z) \mid t \subseteq t_{\vec z}] \geq \delta$ can be checked in linear time. %To sum up:

\begin{proposition}\label{prop:probabilisticreasonDT}
Let $T \in \dt_n$ and $\vec{x} \in \{0,1\}^n$ such that $T (\vec{x}) = 1$.
Then, finding a $\delta$-probable reason for $\vec x$ given $T$ can be done in $O(n\size{T})$ time.
\end{proposition}

Unfortunately, this result cannot be extended to the case of random forests:

\begin{proposition}\label{prop:probabilisticreasonRF}
    Let $F \in \rf_{n,m}$ and $\vec x \in \{0,1\}^n$ such that $F(\vec x) = 1$.
%    Unless {\sf P = NP}, there is no polynomial-time algorithm for computing a $\delta$-probable reason for $\vec x$ given $F$.
 Computing a $\delta$-probable reason for $\vec x$ given $F$ is {\sf \#P}-hard.
\end{proposition}

% From this proposition, we can easily design a polynomial-time greedy algorithm for deriving a $\delta$-approximate reason 
% for any instance $\vec{x}$ given a decision tree $T$ (this algorithm is very close to the one used for deriving a sufficient reason, which
% is sketched above).
%sketched in the proof of Proposition \ref{prop:onesufficientRF}).
